# Supplementary material for: Behind the Scenes: On the Relationship Between Developer Experience and Refactoring
Source: arXiv:2109.11089 source file (2021-09-23)
Supplement: Supplementary file 1 [file SI_Requirement.pdf]

Journal of Software: Evolution and Process

# Special Issue on
# Software Refactoring: Application Breadth and Technical Depth

## Call for Papers

Successful software products evolve through a process of continuous change as bugs are fixed, new features added, and quality issues addressed. Often, software changes are performed by developers who are not the original code authors. Poorly planned changes typically lead to poor design quality, which can result in reduced productivity, decreased system performance, increased fault-proneness, thus making software costly to develop and maintain.

Refactoring supports the dynamic software lifecycle by providing better ways to reduce and manage the growing complexity of software while improving developer productivity. Refactoring can be performed at all levels from requirements to design, architecture and source code level. In essence, it involves improving the internal structure of a software artifact without altering its functionality.

Due to the growing complexity of software systems, in the last ten years we have seen a dramatic increase and industry demand for tools and techniques on software refactoring. In spite of the popularity of refactoring both in practice and as a research topic, many open questions remain, to name a few, understanding how refactoring is performed, measuring the impact of refactoring on software evolution and quality, and improving tool support in all areas of refactoring beyond refactoring recommendation.

The Special issue on Software Refactoring: Application Breadth and Technical Depth is an initiative to promote software refactoring research and practice to the next level. The focus of this special issue is to provide an opportunity for the researchers and practitioners in academia and industry to present novel applications and areas of research as well as new empirical results and insights, and to present new techniques and tool support for advancing software refactoring practices and its impact. In this special issue we both invite extended versions of the best papers presented at IWoR 2020, and solicit novel submissions related to software refactoring. The list of topics includes but not limited to:

- Source code refactoring

- Requirement, design and architecture refactoring
- Refactoring opportunities detection and recommendation
- Tool support for refactoring
- Mining and analyzing refactoring changes
- Code smell detection and remedy
- Effect of refactoring on system complexity and quality
- Refactoring to pattern
- Machine learning driven refactoring
- Refactoring of mobile, web and cloud applications
- Roles of refactoring in software evolution and maintenance

## Important Dates

- Submission deadline: January 15, 2021
- First notification: April 9, 2021
- Revision submission: July 9, 2021
- Notification of acceptance: September 10, 2021

## Submission Guidelines:

Authors should prepare their manuscript according to the Guide for Authors of the Software: Evolution and Process. The submission site is http://mc.manuscriptcentral.com/jsme. Please select "**Software Refactoring**" in the submission system. All the papers will be peer-reviewed following the Software: Evolution and Process reviewing procedures. Submitted manuscripts should not have been published previously, nor be under consideration for publication elsewhere. If the submission is an extended work of a previously published conference /workshop paper, you must submit a cover letter/document detailing (1) the "Summary of Differences" between the Conference/workshop paper and extended version paper, (2) a clear list of "new and original" ideas/contributions in the extended version paper (identifying sections where they are proposed/presented), (3) confirmation of the percentage of new material (at least 30%), and (4) the previously published conference/workshop paper.

## Guest Editors:

**Zhenchang Xing, PhD**
Corresponding Guest Editor
Associate Professor
Research School of Computer Science
Australian National University
Email: zhenchang.xing@anu.edu.au

**Gennadiy Civil**
Software Engineering Manager, Google
Adjunct Professor, Software Engineering, New York University
Email: misterg@google.com

## Guest Editors Short CV

**Dr. Zhenchang Xing** is an Associate Professor in the Research School of Computer Science, Australian National University. Previously, he was an Assistant Professor in the School of Computer Science and Engineering, Nanyang Technological University, Singapore, from 2012-2016. Before joining NTU, Dr. Xing was a Lee Kuan Yew Research Fellow in the School of Computing, National University of Singapore from 2009-2012. Dr. Xing's current research area is in the inter-disciplinary areas of software engineering, human-computer interaction and applied AI. Dr. Xing has over 140 publications in peer-refereed journals and conference proceedings, and have received several distinguished paper awards from top software engineering conferences. Dr. Xing regularly serves on the organization and program committees of the top software engineering conferences. He is the program committee co-chair for ICSME2020 and the associate editor of the Journal of Software: Evolution and Process.

**Gennadiy Civil** is a Software Engineering Manager at Google New York City, USA with over 26 years of industry experience and a particular interest in Software Evolution and

Refactoring practices. He also teaches Software Engineering at NYU. http://www.linkedin.com/in/gcivil
